# Supplementary material for: Self-Blinding and Counterfactual Self-Simulation Mitigate Biases and Sycophancy in Large Language Models
Source: arXiv:2601.14553 source file (2026-01-21)
Supplement: Supplementary file 1 [file model-size.tex]

\section{Issues Generalize Across Model Families and Model Sizes}
\label{sup:model-size}

While we focus on two models in particular -- Qwen2.5-7B-Instruct and GPT-4.1 -- the behavior we observe is by no means unique to these two models or model families.

Both sycophancy and demographic bias are widely documented issues in LLMs, but here we present evidence showing that the problems we report with Qwen2.5-7B-Instruct and GPT-4.1 appear in a wide range of LLMs and are not specific to any particular model, model family, model provider, or model size.
